# Supplementary material for: Message-Passing Algorithms and Homology
Source: arXiv:2009.11631 source file (2020-09-24)
Supplement: Supplementary file 1 [file legendre.tex]

\section{Legendre Transform.}
\renewcommand{\k}{\mathcal{C}}
\newcommand{\vv}{\mathfrak{v}}
\newcommand{\kint}{\mathring{\mathcal{C}}}

Consider a convex subset of some vector space $\k \incl \vv$. 
Denote by $\vv_\k \incl \vv$ the vector space spanned by $\k$
and by $\kint$ the interior of $\k$ for the induced topology on $\vv_\k$.
By convexity, $\kint$ is an open submanifold of $\vv_\k$ of maximal dimension 
and we identify $T\kint$ with $\kint \times \vv_\k$. 

Let $F$ denote a smooth convex function on $\k$.
The image of its differential $F_*(\kint)$ 
is a convex subset of linear forms in $\vv^*_\k$.
We denote by $\tilde{\k} \incl \vv^*$ its reciprocal image under the projection
$\vv^* \aw \vv_\k^* \sim \vv^* / \vv_\k^\perp$:
\begin{equation} \tilde{\k} = F_*(\kint) + \vv_\k^\perp \end{equation}
The Legendre transform of $F$ is a convex function 
$\tilde{F}$ defined on $\tilde{\k}$ whose construction we briefly recall.

Consider the smooth function $L_F : \vv^* \times \kint \aw \R$ defined by:
\begin{equation} L_F(u,v) = F(v) - \croc{u}{v}  \end{equation}
For every $u \in \vv^*$, $L_F(u, \,\cdot\,)$ is still
a convex function on $\kint$, 
it reaches a global minimum if and only if the restriction
of its differential to $\vv_\k$ vanishes on some critical point. 
Such a critical point $v \in {\frak v}$ satisfies $F_*(v) \in u + \vv_\k^\perp$.
It follows that $L_F(u,\,\cdot\,)$ reaches a global minimum on $\kint$ 
if and only if $u \in \tilde{\k}$.

The Legendre transform of $F$ is defined for every $u \in \tilde{\k}$ as:
\begin{equation} \tilde{F}(u) = \min_{v \in \kint} L_F(u,v) \end{equation}
One has $\tilde{F}(u) = F(v) - \croc{u}{v}$ for every $v$ such that
$F_*(v) \in u + \vv_\k^\perp$.
It follows that if $u' = u + n$ with $n \in \vv_\k^\perp$,
then $\tilde{F}(u') = \tilde{F}(u) - \croc{n}{v}$. 
In particular, $\tilde{F}_*$ is constant along $\vv_\k^\perp$.

It can be shown that this transformation is involutive, so that one recovers 
$F : \kint \aw \R$ by applying the previous construction to 
$\tilde{F} : \tilde{\k} \aw \R$.
