# Supplementary material for: Message-Passing Algorithms and Homology
Source: arXiv:2009.11631 source file (2020-09-24)
Supplement: Supplementary file 2 [file category.tex]

\section{Category Theory}
